# Supplementary material for: NBNet: Noise Basis Learning for Image Denoising with Subspace Projection
Source: arXiv:2012.15028 source file (2021-05-11)
Supplement: Supplementary file 1 [file fig_supp_basis.tex]

\begin{figure*}[ht]
    \begin{subfigure}{}
    \centering
    \scalebox{1}{
    \begin{tabular}[b]{c@{ } c@{ }  }%\hspace{-2.4mm}
         \multirow{4}{*}{\includegraphics[width=.33\textwidth,valign=tl]{pic/basis/259_svd.jpg}} 
        &  \includegraphics[width=.152\textwidth,valign=t]{pic/basis/258_noisy.jpg}

        \vspace{0.5mm}
    \\
        &  Noisy   \\
 
        &\includegraphics[width=.152\textwidth,valign=t]{pic/basis/259_gt.jpg}  
        
         \\
    
          Visualization of basis & Reference 
         \\
         \multicolumn{2}{c}{(a)}
         \\
    
    \end{tabular}}
    \end{subfigure}
    \begin{subfigure}{}
    \centering
    \scalebox{1}{
    \begin{tabular}[b]{c@{ } c@{ } 	}%\hspace{-2.4mm}
         \multirow{4}{*}{\includegraphics[width=.33\textwidth,valign=tl]{pic/basis/485_svd.jpg}} 
        &  \includegraphics[width=.152\textwidth,valign=t]{pic/basis/485_noisy.jpg}

        \vspace{0.5mm}
    \\
        &  Noisy   \\
 
        &\includegraphics[width=.152\textwidth,valign=t]{pic/basis/495_gt.jpg}  
        
         \\
    
          Visualization of basis & Reference 
         \\
         \multicolumn{2}{c}{(b)}
         \\
               
    \end{tabular}}
    \end{subfigure}
    \vspace{-3mm}
    \caption{\small {(a) and (b) are basis visualization of different input image.
    } }
    \label{fig:basis vector visual supp1}
    
 \end{figure*}
