# Supplementary material for: NBNet: Noise Basis Learning for Image Denoising with Subspace Projection
Source: arXiv:2012.15028 source file (2021-05-11)
Supplement: Supplementary file 2 [file fig_supp_basis2.tex]

\begin{figure}[b]
    \begin{center}
    \begin{subfigure}
    \begin{center}
    
    \tiny
    \scalebox{0.9}{
    \begin{tabular}[b]{c@{ } c@{ }  c@{ } c@{ } c@{ }	}%\hspace{-2.4mm}
         \multirow{4}{*}{\includegraphics[width=.32\textwidth,valign=tl]{pic/basis/485_svd.jpg}} 
        &  \includegraphics[width=.152\textwidth,valign=t]{pic/basis/485_noisy.jpg}

        \vspace{0.5mm}
    \\
        &  Noisy   \\
 
        &\includegraphics[width=.152\textwidth,valign=t]{pic/basis/495_gt.jpg}  
        
         \\
    
          Visualization of basis & Reference 
         \\
               
    \end{tabular}}
    \end{center}
    \end{subfigure}
    \end{center}
    \vspace{-6mm}
    \caption{\small {caption
    } }
    \label{fig:basis vector visual supp2}
    
 \end{figure}
